# Supplementary material for: Coupled nuclear and electron dynamics in the vicinity of a conical intersection
Source: arXiv:2102.13547 ancillary file (2021-02-26)
Supplement: Supplementary file 1 [file si.pdf]

**Supporting Information: Controlling the nuclear- and electron-dynamics at a conical intersection**

Thomas Schnappinger and Regina de Vivie-Riedle

*Department of Chemistry, LMU Munich, Germany, D-81377 Munich, Germany*

(Dated: 14 December 2020)

## CONTENTS

|                                                         |           |
|---------------------------------------------------------|-----------|
| <b>I. Wave-packet Simulation Setup</b>                  | <b>3</b>  |
| <b>II. Quantum chemical data of NO<sub>2</sub></b>      | <b>6</b>  |
| <b>III. NEMol simulations of NO<sub>2</sub></b>         | <b>9</b>  |
| A. NEMol free propagation                               | 10        |
| B. NEMol propagation with CEP laser pulse               | 15        |
| <b>IV. Influence of the TDM on the Waveform control</b> | <b>23</b> |
| <b>References</b>                                       | <b>25</b> |

## I. WAVE-PACKET SIMULATION SETUP

The quantum dynamical simulations were performed by solving the time dependent Schrödinger equation (TDSE)

$$i\hbar \frac{\partial}{\partial t} \Psi = \hat{H} \Psi, \quad (\text{S1})$$

$$\text{with } \hat{H} \Psi = \begin{pmatrix} \hat{T}_q + \hat{V}_0 & \tau_{01} - \mu_{01}\epsilon(t) \\ \tau_{01} - \mu_{01}\epsilon(t) & \hat{T}_q + \hat{V}_1 \end{pmatrix} \begin{pmatrix} \Psi_0 \\ \Psi_1 \end{pmatrix}. \quad (\text{S2})$$

with the kinetic energy operator  $\hat{T}_q$  of the nuclei in internal coordinates  $q$ , the potential energy operator  $\hat{V}$  of the respective state. The kinetic energy operator in internal coordinates is set up according to the G-Matrix formalism<sup>S1-S3</sup> as described in Ref.<sup>S4</sup>. It reads

$$\hat{T}_q \approx -\frac{\hbar^2}{2m} \sum_{r=1}^M \sum_{s=1}^M \frac{\partial}{\partial q_r} \left[ G_{rs} \frac{\partial}{\partial q_s} \right] \quad (\text{S3})$$

with the G-Matrix being computed via its inverse elements

$$(G^{-1})_{rs} = \sum_{i=1}^{3N} m_i \frac{\partial x_i}{\partial q_r} \frac{\partial x_i}{\partial q_s}, \quad (\text{S4})$$

i.e. via finite differences by displacement of the Cartesian molecular geometry along the internal coordinates. The off-diagonal elements of the Hamiltonian include the non-adiabatic coupling NAC's  $\tau_{01}$  which have in general the following form.<sup>S5,S6</sup>

$$\tau_{01} = \langle \Psi_0^{adi} | \nabla | \Psi_1^{adi} \rangle \nabla + \frac{1}{2} \langle \Psi_0^{adi} | \nabla^2 | \Psi_1^{adi} \rangle$$

Since the  $\nabla^2$  term is much smaller than the  $\nabla$  term, it can be neglected in first approximation. However, this would lead to a non-Hermitian Hamiltonian. To avoid this, the non-Hermitian behaviour can be compensated for by using the partition eq. S5<sup>S7,S8</sup>. Here the term  $\langle \nabla \Psi_0^{adi} | \nabla \Psi_1^{adi} \rangle$  can be neglected without loosing the hermiticity.

$$\langle \Psi_0^{adi} | \nabla^2 | \Psi_1^{adi} \rangle = \nabla \langle \Psi_0^{adi} | \nabla | \Psi_1^{adi} \rangle - \langle \nabla \Psi_0^{adi} | \nabla \Psi_1^{adi} \rangle. \quad (\text{S5})$$

Beside the NAC's also the transition dipole moments  $\mu_{01}$  (TDM) between the two relevant electronic states are part of the used Hamiltonian. So the light-matter interaction is treated within the dipole approximation and we are assuming an optimal alignment of the

transition dipole moment and the electric component of the pulse. The few-cycle pulse has a Gaussian shape and is defined as:

$$E(t) = E_{max} \cdot e^{-2\left(\frac{t-t_0}{\sigma}\right)^2} \cdot \cos(\omega_0(t-t_0) + \phi), \quad (\text{S6})$$

with  $\sigma = \frac{\text{FWHM}}{\sqrt{2 \log(2)}}$ .

with the central frequency  $\omega_0$ , the time zero  $t_0$ , the maximal intensity  $E_{max}$ , the full width half maximum (FWHM) and the carrier envelope phase  $\phi$  (CEP).

All molecular quantities (PES's, NAC's, TDM and the G-Matrix) are represented on a two-dimensional spatial grid with 256x256 grid points. The two coordinates spanning the PES's are the gradient difference and derivative coupling vectors defining the branching space of the  $D_1/D_0$ -CoIn of the  $\text{NO}_2$  molecule. These two vectors correspond to the bending angle  $\alpha$  and the asymmetric stretching coordinate  $b$ , defined as half the difference between the two NO distances. The last internal degree of freedom, the symmetric stretch coordinate, is kept constant at the value of the optimized  $D_1/D_0$ -CoIn (1.267 Å). The corresponding G-Matrix elements are shown in FIG. S1.

The quantum dynamical simulations are conducted with a program developed in our own group. The numerical propagation on the adiabatic potential energy surfaces (PES's) is performed by integration of the TDSE according to

$$\Psi(t+dt) = e^{(-i\hat{H}dt)}\Psi(t) = \hat{U}\Psi(t). \quad (\text{S7})$$

The evolution operator  $\hat{U}$  is expanded in a Chebyshev series<sup>S9</sup>. For all simulations a time step of 0.5 a.u. is used. The total simulation time was 60 fs. The propagations were started by assuming a delta pulse excitation.

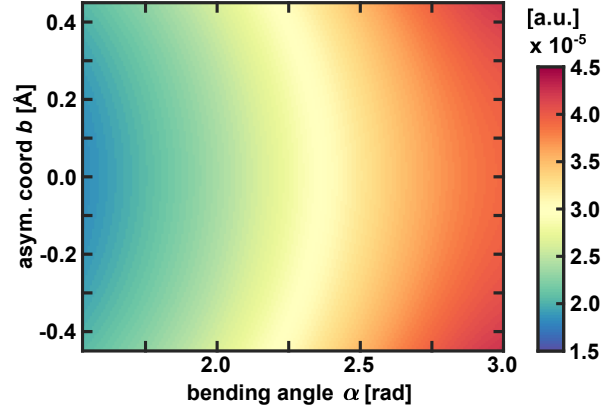

(a)

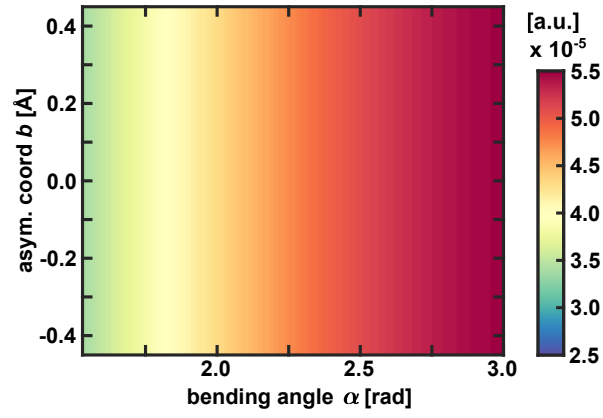

(b)

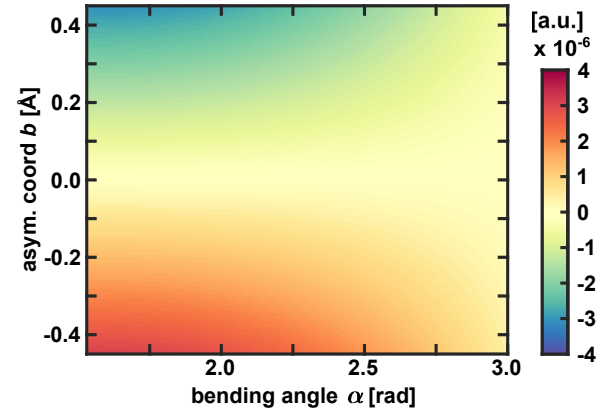

(c)

FIG. S1. : G-matrix elements setting up the kinetic energy operator for the quantum dynamical simulations. (a) G11  $\alpha$ -coordinate (b) G22  $b$ -coordinate (c) G12 kinetic coupling.

## II. QUANTUM CHEMICAL DATA OF NO<sub>2</sub>

The PES's, the TDM and the NAC's for the NO<sub>2</sub> molecule were computed with the state-average complete active space self-consistent field method<sup>S10,S11</sup> including five states in the state-averaging procedure (SA5-CASSCF). All calculations were carried out with the MOLPRO 2012.1<sup>S12,S13</sup> program package and the basis set 6-311G\* was used. An active space including thirteen electrons in ten orbitals (AS(13,10)) (see FIG. II) was employed.

In TABLE S1 the electronic character and the vertical excitation energy  $\Delta E$  of the first three Doublet states are listed for all relevant critical points. The geometric parameters of the optimized critical points (minima and conical intersection) are shown in TABLE S2.

TABLE S1. Electronic character and vertical excitation energy  $\Delta E$  at all relevant critical points of NO<sub>2</sub> on the SA5-CASSCF/6-311G\* level of theory.

|                          | state | character | $\Delta E$ [eV] |
|--------------------------|-------|-----------|-----------------|
| optimized $D_0$ minimum  | $D_0$ | $n_N$     | 0.000           |
|                          | $D_1$ | $n_O$     | 3.222           |
|                          | $D_2$ | $n_O$     | 3.231           |
| optimized $D_1$ minimum  | $D_0$ | $n_O$     | 1.164           |
|                          | $D_1$ | $n_N$     | 1.798           |
|                          | $D_2$ | $n_O$     | 2.034           |
| optimized $D_1/D_0$ CoIn | $D_0$ | $n_O$     | 1.226           |
|                          | $D_1$ | $n_N$     | 1.226           |
|                          | $D_2$ | $n_O$     | 1.884           |

TABLE S2. Geometric parameters for the relevant critical points of NO<sub>2</sub> optimized on the SA5-CASSCF/6-311G\* level of theory.

|                          | $\alpha$ [rad] | $r_{NO1}$ [Å] | $r_{NO2}$ [Å] | $b$ [Å] |
|--------------------------|----------------|---------------|---------------|---------|
| optimized $D_0$ minimum  | 2.328          | 1.208         | 1.208         | 0.000   |
| optimized $D_1$ minimum  | 1.782          | 1.273         | 1.273         | 0.000   |
| optimized $D_1/D_0$ CoIn | 1.876          | 1.267         | 1.267         | 0.000   |

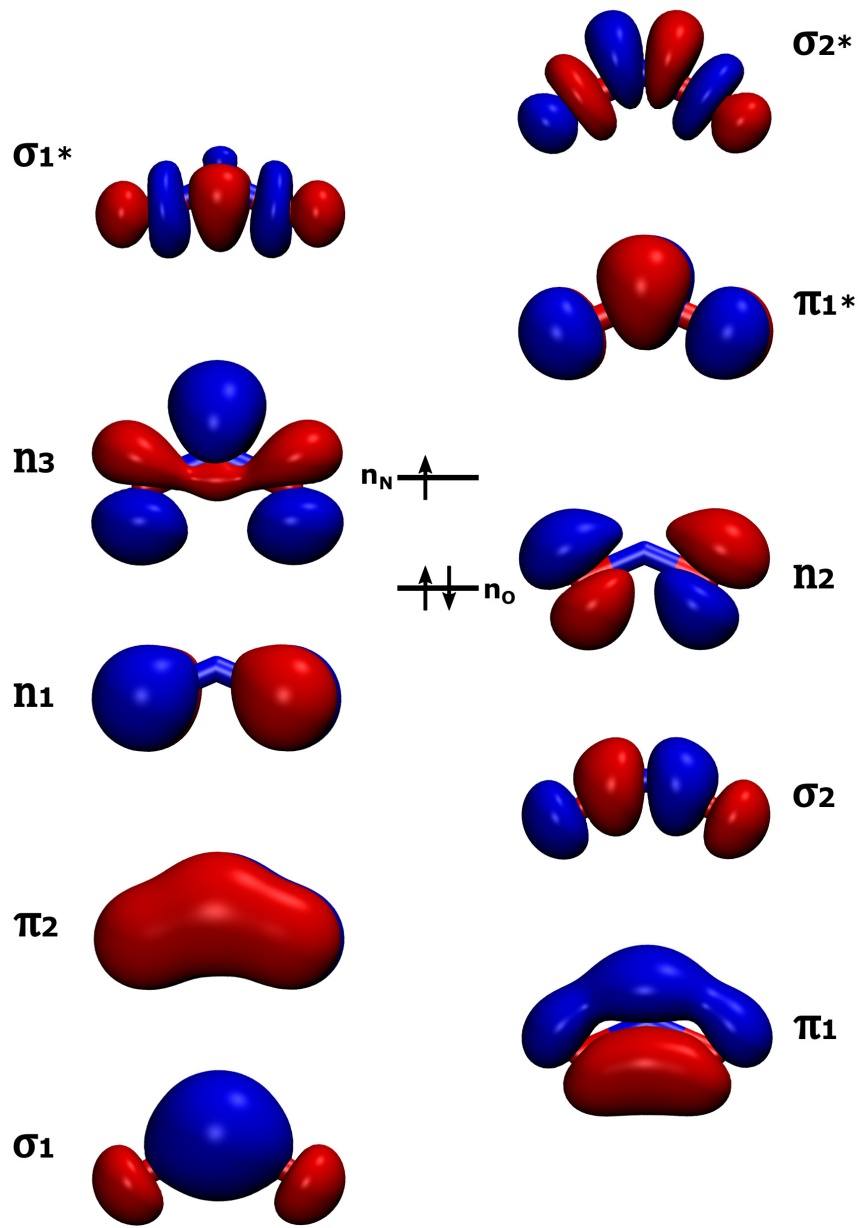

FIG. S2. SA5-CASSCF molecular orbitals included in the active space AS(13/10) of  $\text{NO}_2$ , obtained using the 6-311G\* basis set at optimized  $D_0$  minimum. The orbitals are rendered with an isovalue of 0.05.

The CASSCF minima and the CI geometry are very close to the experimental structures found in literature<sup>S14–S16</sup> and also in close coincide with previous MR-CISD results<sup>S17</sup>.

In order to obtain the adiabatic surfaces of the  $D_0$  and the  $D_1$  state all other states were diabaticized with respect to these two states. For the diabaticization a number of schemes

based on different approaches have been developed, for an overview see Ref.<sup>S18</sup>. In the present study, the diabaticization was performed using a procedure based on the adiabatic diople and transient-dipole moments, for details see Refs.<sup>S19–S21</sup>.

The absolute value of the transient-dipole moment vector and its corresponding  $y$ - and  $z$ -element are shown in FIG. S3

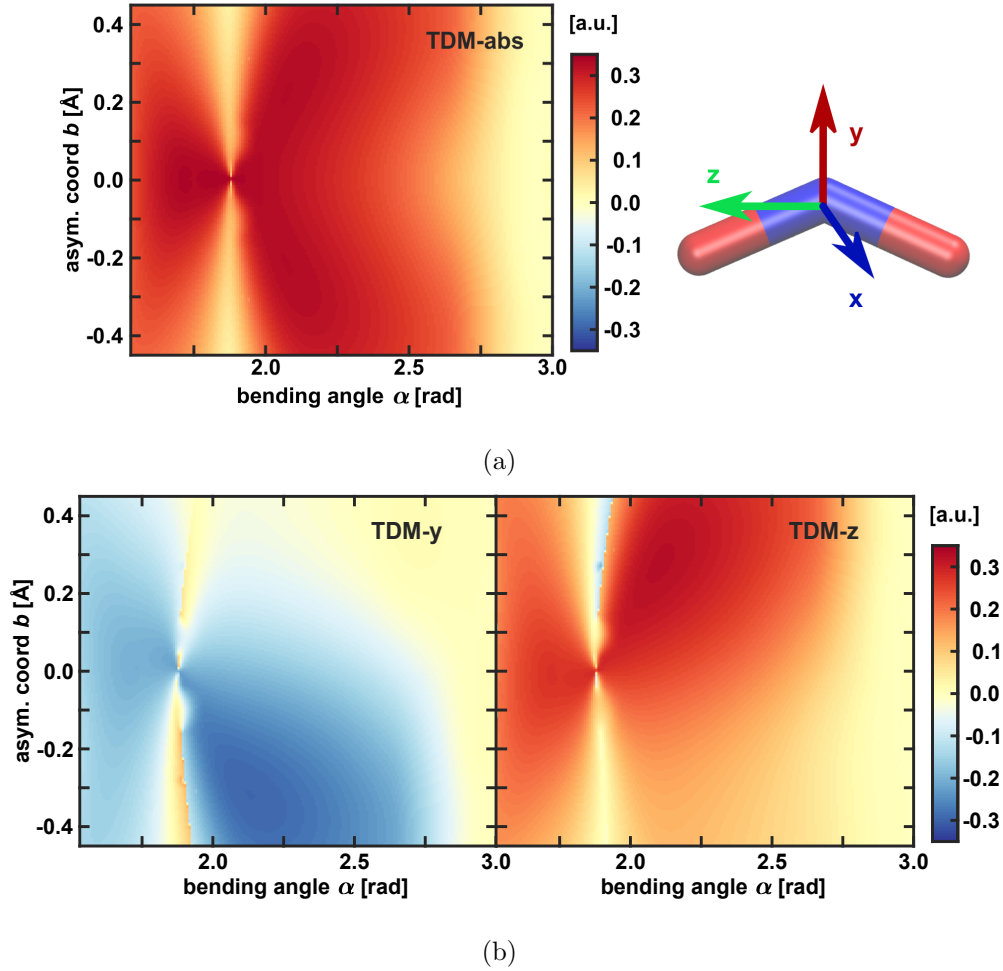

FIG. S3. (a) Absolute value of the  $D_1$ - $D_0$  transition dipole moment. (b) The  $y$ -element (left) and the  $z$ -element (right) of the transition dipole moment vector. For the orientation of the molecule see top right.

### III. NEMOL SIMULATIONS OF NO<sub>2</sub>

The NEMol-grid consists of  $15 \times 13$  points which are equally distributed between 1.34 rad to 2.86 rad in the  $\alpha$ -coordinate and between  $-0.33 \text{ \AA}$  to  $0.33 \text{ \AA}$  in the  $b$ -coordinate. The energy difference  $\Delta E$  between the  $D_0$  and  $D_1$  state for each grid point of the NEMol-grid is shown in FIG. S4.

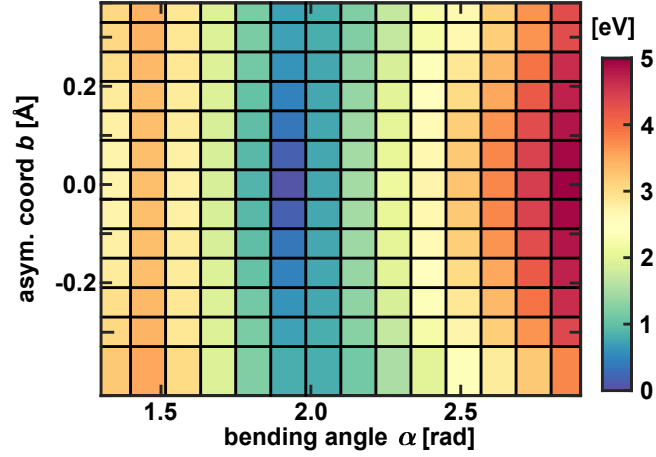

FIG. S4. Energy difference  $\Delta E$  between the  $D_0$  and  $D_1$  state represented on the NEMol-grid.

## A. NEMol free propagation

The temporal evolution of the probability density on the  $D_0$  and  $D_1$  surface integrated over the  $\alpha$ -coordinate respectively the  $b$ -coordinate are depicted in FIG. S5.

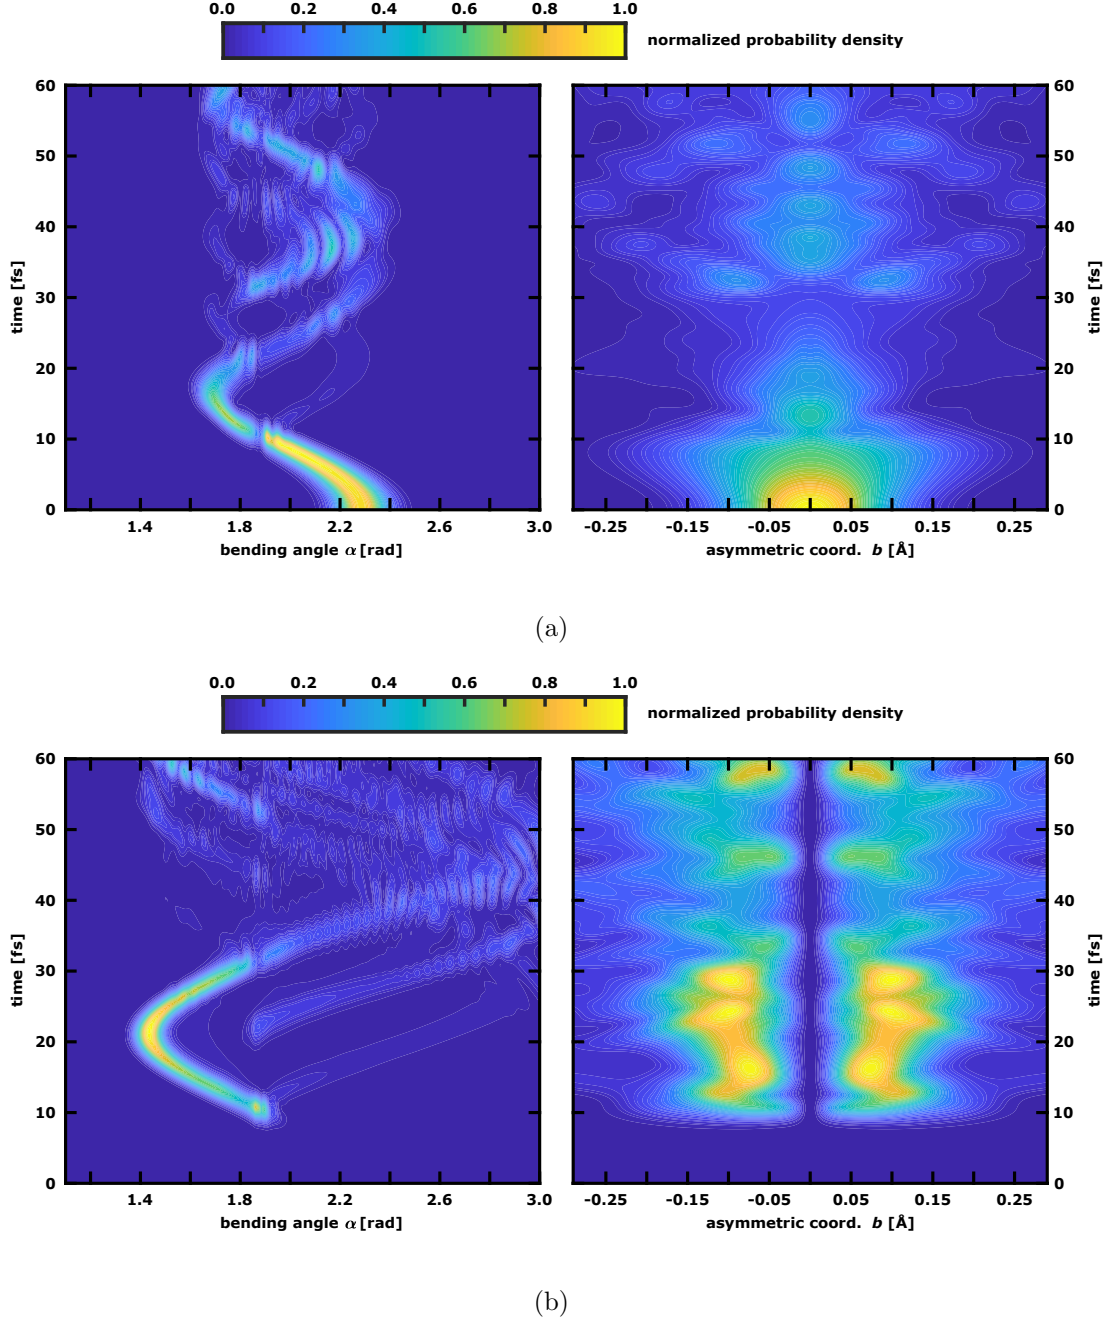

FIG. S5. Nuclear probability density evolution on the adiabatic  $D_1$ -surface (a) (left integrated over the  $b$ -coordinate and right integrated over the  $\alpha$ -coordinate) and on the adiabatic  $D_0$ -surface (b) (left integrated over the  $b$ -coordinate and right integrated over the  $\alpha$ -coordinate).

The transformation of the full wave-packet in the field-free case onto the NEMol-grid, the overlap terms and the resulting coherence terms are visualized in FIG. S6 for four points in time (0 fs, 9 fs, 13 fs, 20 fs).

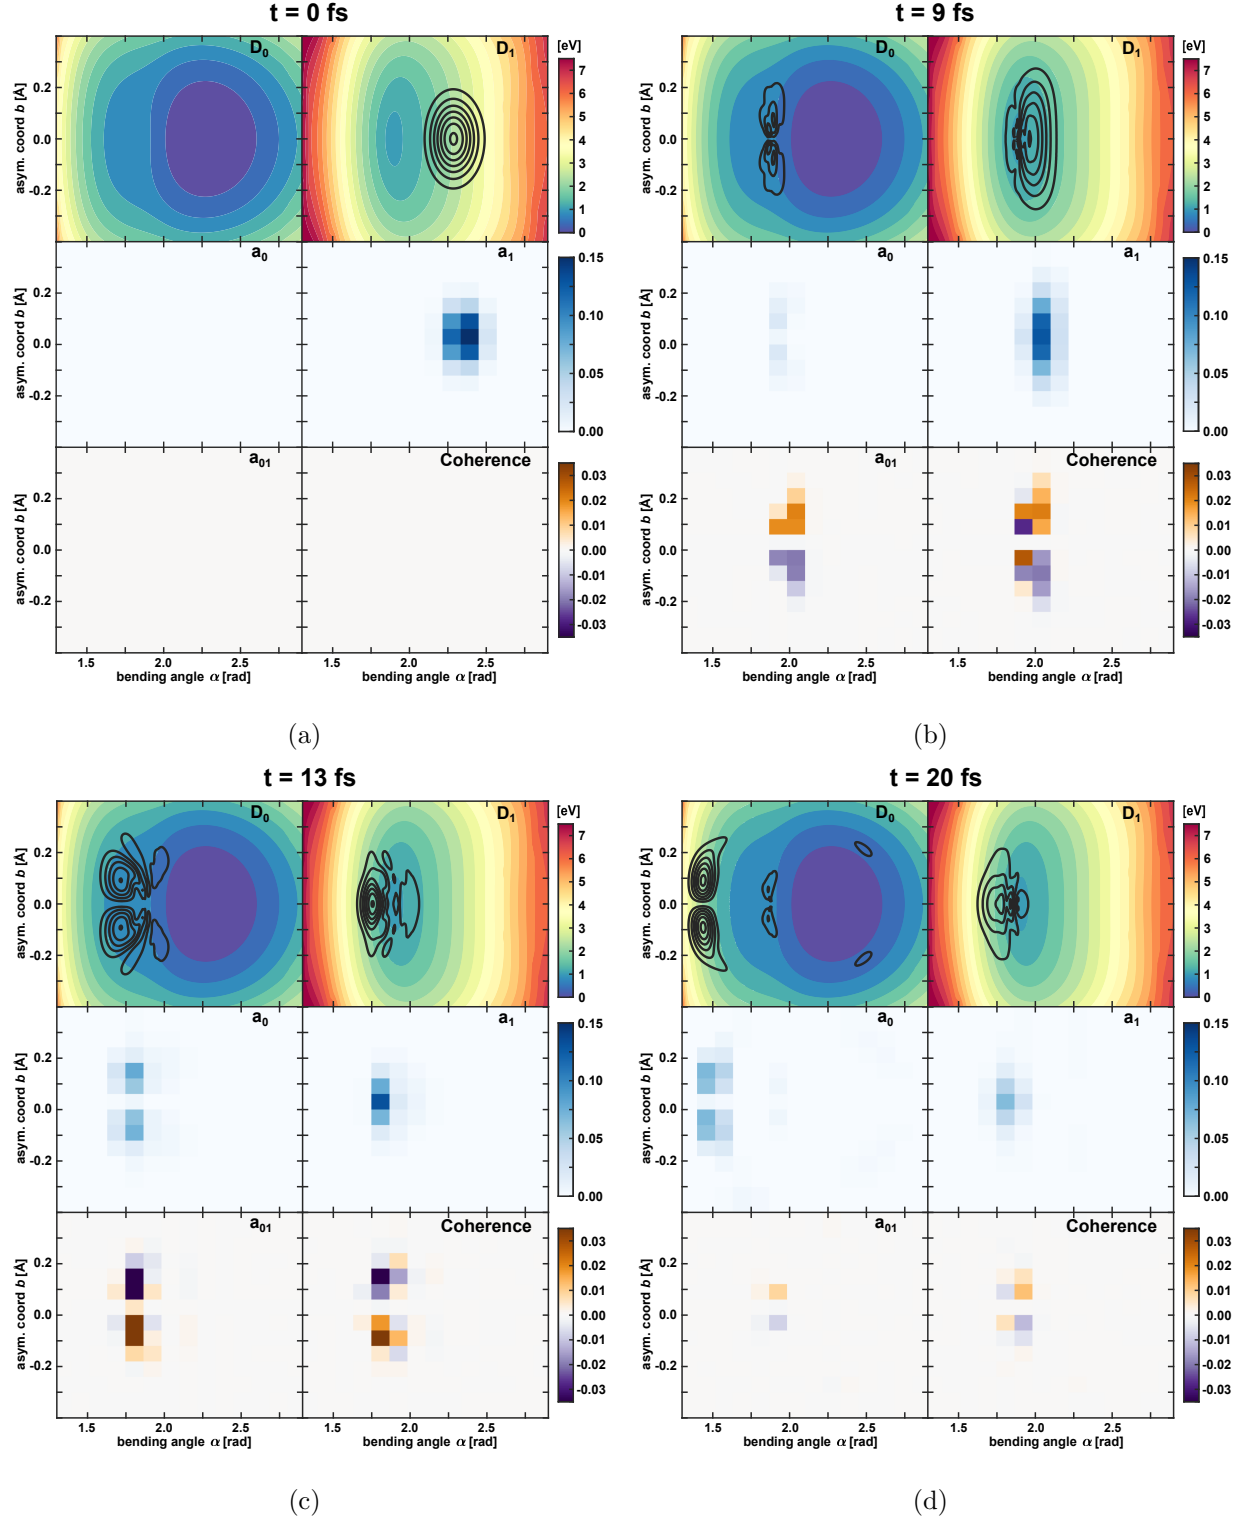

FIG. S6. Top: Visualization of the wave packet on the coupled PES. Middle: Population  $a_0$  and  $a_1$  on the NEMol-gird. Bottom: Tow-times the real-valued parts of the overlap  $a_{01}$  and of the full Coherence term. All values are shown for 0 fs (a), 9 fs (b), 13 fs (c), 20 fs (d).

TABLE S3. Observed frequencies in the dynamics of the  $y$ -DM component. Obtained by Fourier transform of the  $\Delta$ -1e-2o-, the 1e-2o- $y$ -DM component as well as the component calculated with the full density. All values given in eV.

| $\Delta$ -1e-2o- $y$ -DM | 1e-2o- $y$ -DM | full- $y$ -DM |
|--------------------------|----------------|---------------|
| 0.207                    | 0.138          | 0.138         |
| 0.414                    | 0.345          | 0.483         |
| 0.622                    | 0.621          | 0.622         |
| 0.829                    | 0.760          | 0.760         |
| 0.967                    | 0.967          | 1.036         |
| 1.174                    | —              | —             |
| 1.381                    | —              | —             |
| 1.588                    | —              | —             |
| 1.864                    | —              | —             |
| 2.141                    | —              | —             |

The frequencies obtained by Fourier transform of the  $y$ - and  $z$ -component of the dipole moment with an intensity larger than 0.1 can be found in TABLE S3 and TABLE S4.

TABLE S4. Observed frequencies in the dynamics of the  $z$ -component of the dipole moment. Obtained by Fourier transform of the  $\Delta$  1e-2o- , the 1e-2o-component as well as the component calculated with the full density. All values given in eV.

| $\Delta$ 1e-2o- $z$ DM | 1e-2o- $z$ DM | full- $z$ DM |
|------------------------|---------------|--------------|
| 0.207                  | 0.207         | 0.345        |
| 0.483                  | 0.483         | 0.483        |
| 0.691                  | 0.691         | 0.760        |
| 0.898                  | 0.898         | 0.898        |
| 1.105                  | 1.105         | —            |
| 1.243                  | 1.243         | —            |
| 1.450                  | 1.450         | —            |
| 1.657                  | 1.657         | —            |
| 1.795                  | —             | —            |
| 2.072                  | —             | —            |
| 2.279                  | —             | —            |

The interplay of the overlap part (blue) and the phase part (green) of the coherent term in the NEMol-ansatz is illustrated in in FIG. S7 for two individual NEMol-grid points. Since we are forming the product of the overlap and the phase the overall coherent term (red) and thus the frequencies observed are higher than for the individual contributions.

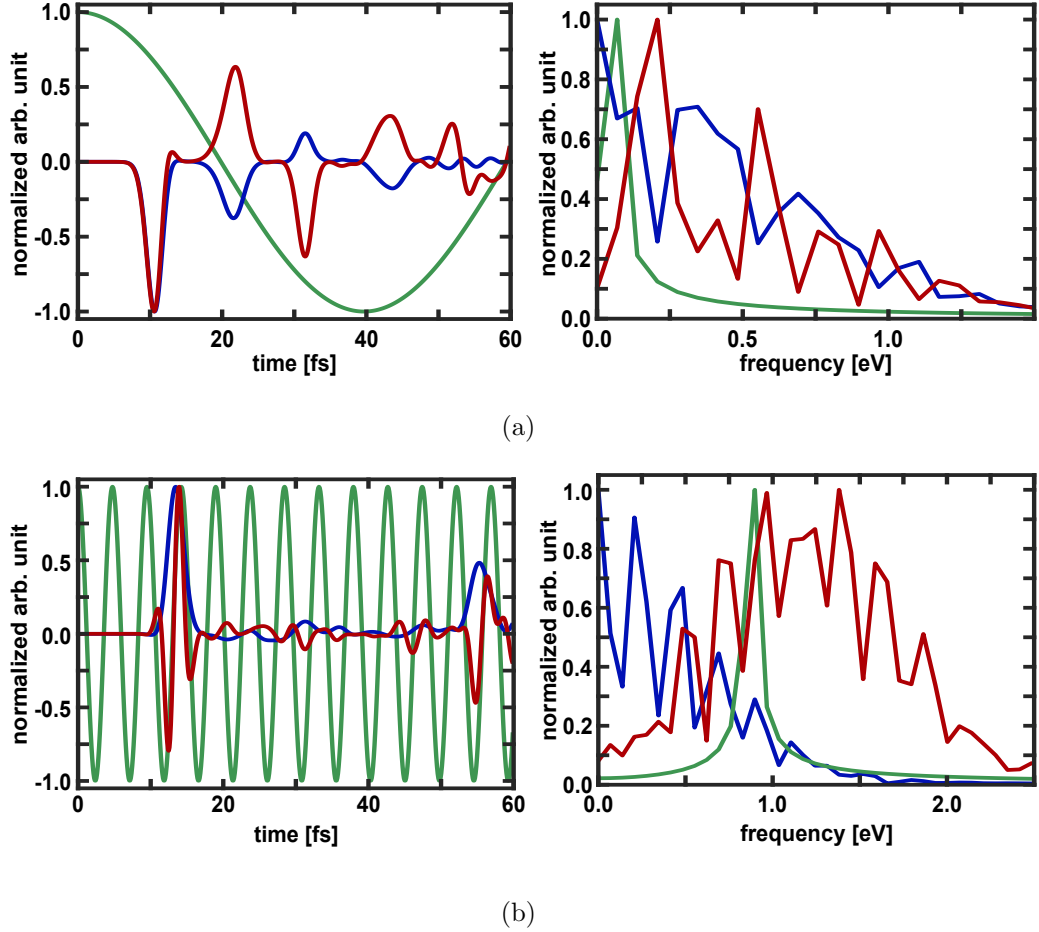

FIG. S7. Temporal evolution and Fourier transformation of two-times the real-valued part of the overlap term (blue), the phase term (green) and the complete coherence term (red) for the (a) grid-window containing the CoIn and (b) a grid-window near the CoIn (one step to smaller  $\alpha$  values).

## B. NEMol propagation with CEP laser pulse

The temporal evolution of the probability density in the presents of a few-cycle IR pulse with different CEP's on the  $D_0$  and  $D_1$  surface integrated over the  $\alpha$ -coordinate respectively

the  $b$ -coordinate are depicted in FIG. S8 and in FIG. S9.

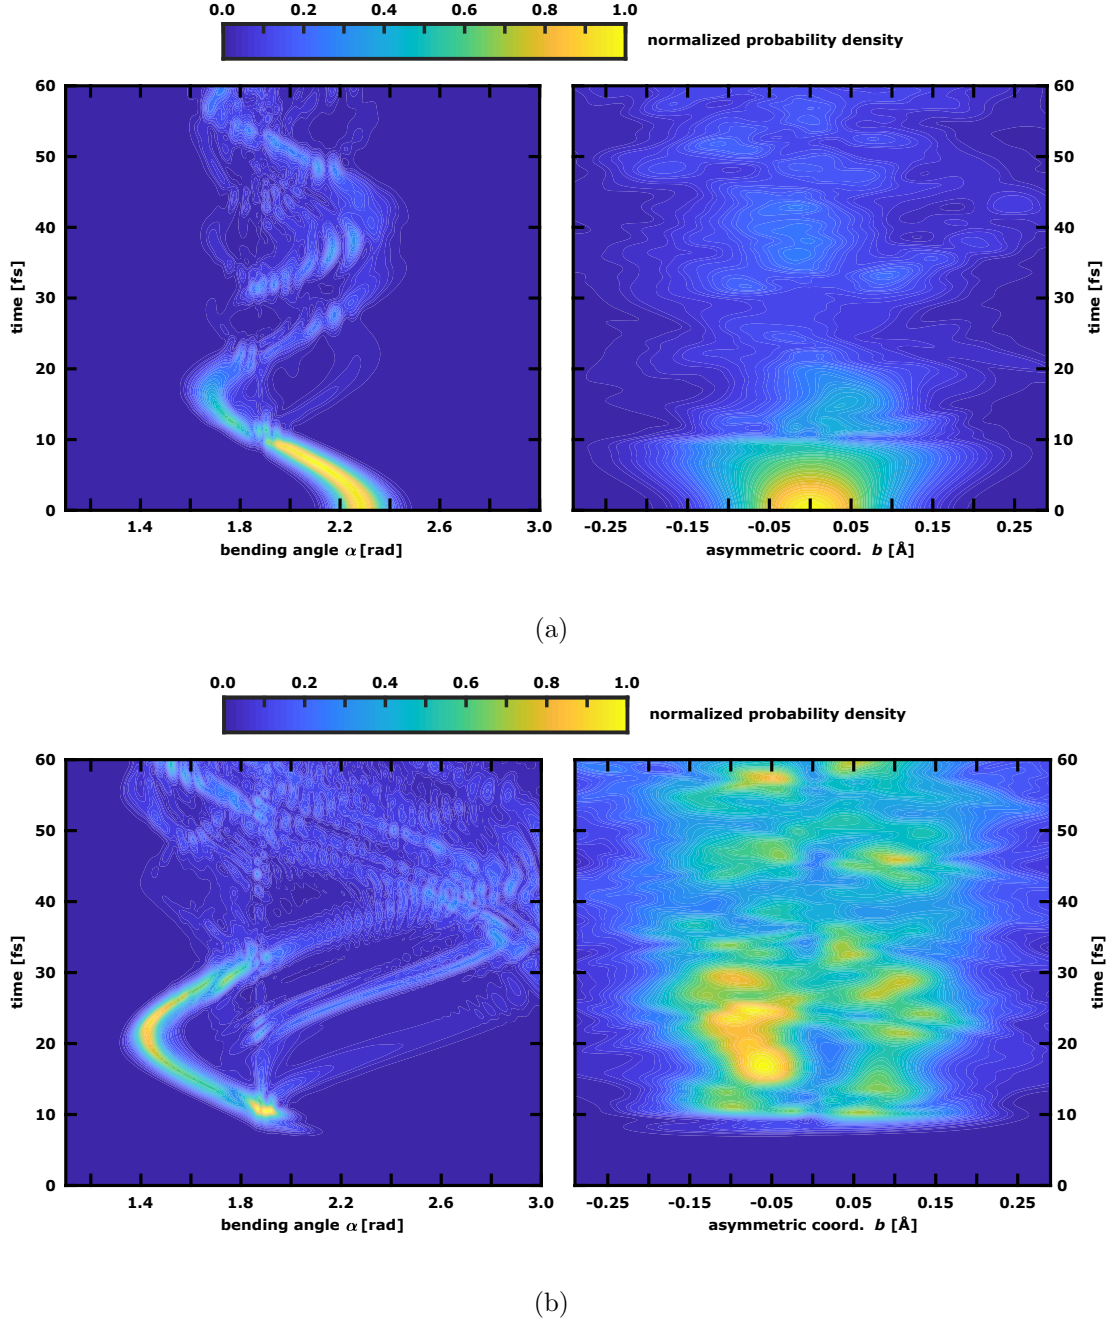

FIG. S8. Nuclear probability density evolution on the adiabatic  $D_1$ -surface (a) (left integrated over the  $b$ -coordinate and right integrated over the  $\alpha$ -coordinate) and on the adiabatic  $D_0$ -surface (b) (left integrated over the  $b$ -coordinate and right integrated over the  $\alpha$ -coordinate). Both in the presents of a few-cycle IR pulse with a CEP of  $0.0\pi$ .

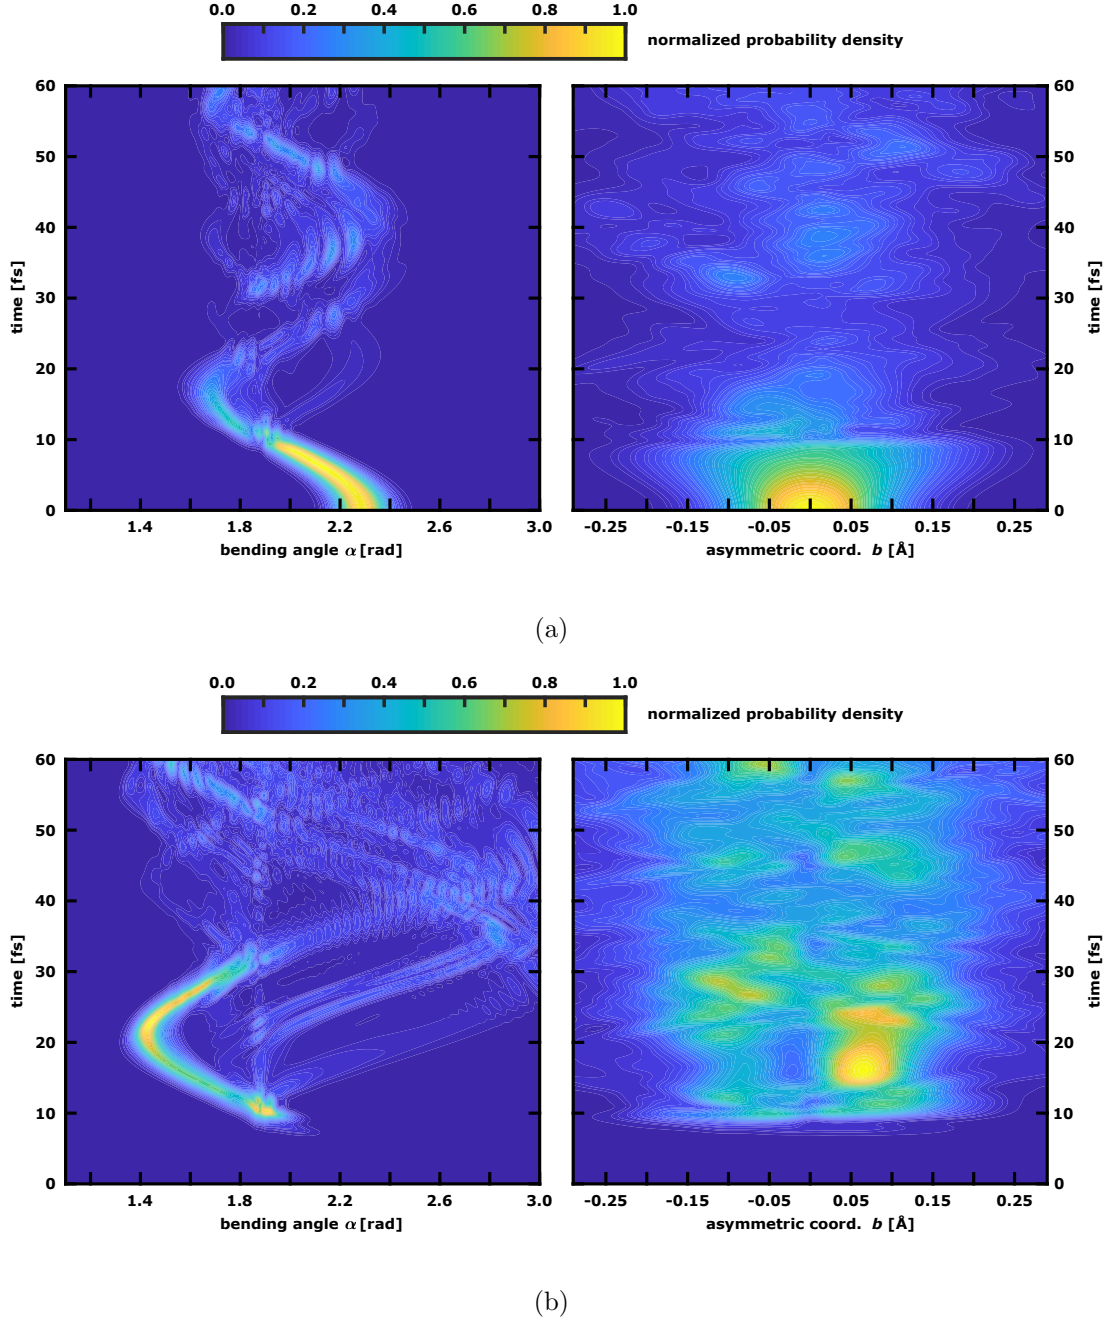

FIG. S9. Nuclear probability density evolution on the adiabatic  $D_1$ -surface (a) (left integrated over the  $b$ -coordinate and right integrated over the  $\alpha$ -coordinate) and on the adiabatic  $D_0$ -surface (b) (left integrated over the  $b$ -coordinate and right integrated over the  $\alpha$ -coordinate). Both in the presents of a few-cycle IR pulse with a CEP of  $1.4\pi$ .

The transformation of the full wave-packet in the presents of a few-cycle IR pulse with a CEP of  $0.0\pi$  onto the NEMol-grid, the overlap terms and the resulting coherence terms are visualized in FIG. S10 for four points in time (9 fs, 11 fs, 13 fs, 20 fs).

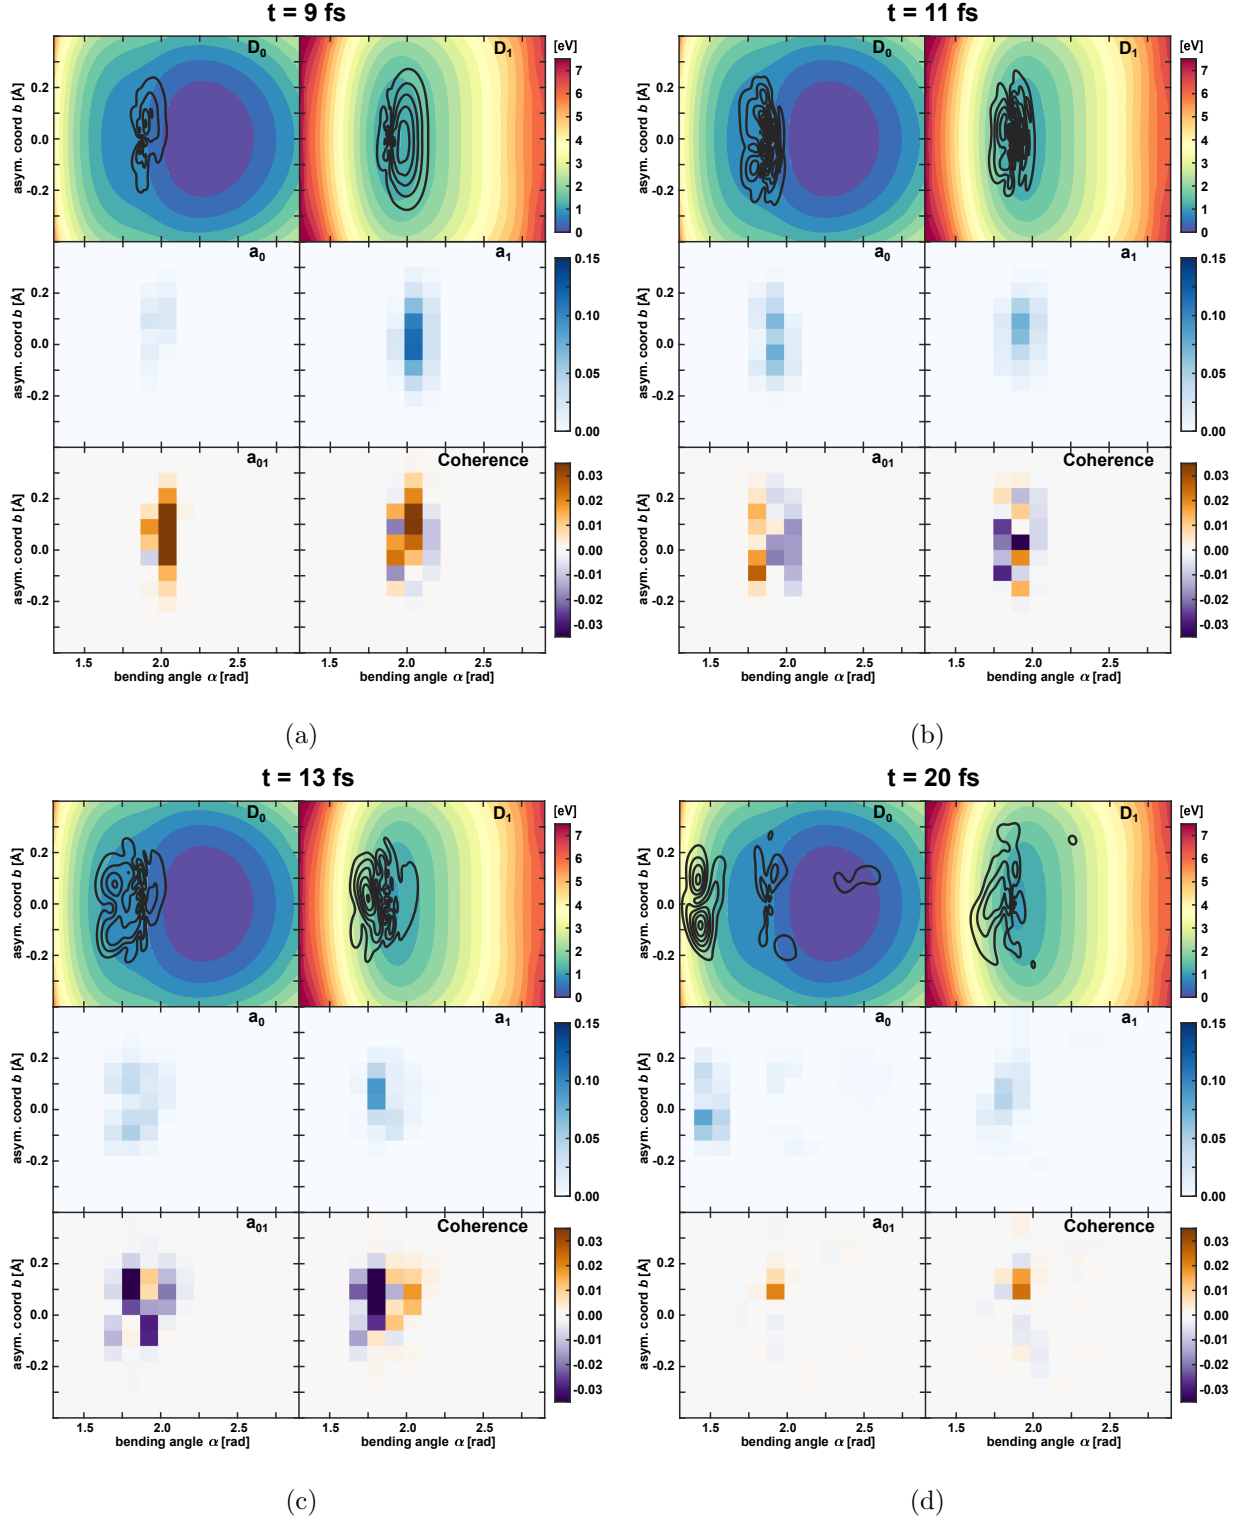

FIG. S10. Top: Visualization of the wave packet in the presents of a CEP-pulse ( $0.0\pi$ ). Middle: Population  $a_0$  and  $a_1$  on the NEMol-gird. Bottom: Tow-times the real-valued part of the overlap  $a_{01}$  and of the full Coherence term. All values are shown for 9 fs (a), 11 fs (b), 13 fs (c), 20 fs (d).

TABLE S5. Observed frequencies of dynamics of the  $y$ -DM component with a few-cycle IR pulse (CEP of  $0.0\pi$ ) included in the simulation. Obtained by Fourier transformation of the  $\Delta$ -1e-2o-, the 1e-2o- $y$ -DM component as well as the component calculated with the full density. All values given in eV.

| $\Delta$ -1e-2o- $y$ -DM | 1e-2o- $y$ -DM | full- $y$ -DM |
|--------------------------|----------------|---------------|
| 0.207                    | 0.138          | 0.138         |
| 0.414                    | 0.345          | 0.483         |
| 0.622                    | 0.621          | 0.622         |
| 0.829                    | 0.760          | 0.760         |
| 0.967                    | 0.967          | 1.036         |
| 1.174                    | —              | —             |
| 1.381                    | —              | —             |
| 1.657                    | —              | —             |
| 1.864                    | —              | —             |
| 2.141                    | —              | —             |
| 2.348                    | —              | —             |
| 2.624                    | —              | —             |
| 2.762                    | —              | —             |
| 2.900                    | —              | —             |
| 3.038                    | —              | —             |
| 3.245                    | —              | —             |
| 3.384                    | —              | —             |
| 3.522                    | —              | —             |
| 3.729                    | —              | —             |
| 4.005                    | —              | —             |
| 4.143                    | —              | —             |

The frequencies obtained by Fourier transform of the  $y$ - and  $z$ -component of the dipole moment in the presents of a CEP-pulse ( $0.0\pi$ ) with an intensity larger than 0.1 can be found in TABLE S5 and TABLE S6.

TABLE S6. Observed frequencies of dynamics of the  $z$ -DM component with a few-cycle IR pulse included in the simulation. Obtained by Fourier transformation of the  $\Delta$  1e-2o-, the 1e-2o- $z$ -DM component as well as the component calculated with the full density. All values given in eV.

| $\Delta$ 1e-2o- $z$ -DM | 1e-2o- $z$ -DM | full- $z$ -DM |
|-------------------------|----------------|---------------|
| –                       | –              | 0.069         |
| 0.207                   | 0.207          | 0.207         |
| 0.345                   | 0.345          | 0.345         |
| 0.483                   | 0.483          | –             |
| 0.760                   | 0.760          | 0.622         |
| 1.036                   | 1.036          | 1.105         |
| 1.243                   | 1.243          | 1.312         |
| 1.519                   | 1.519          | 1.519         |
| 1.726                   | 1.726          | 1.795         |
| 1.864                   | 1.864          | –             |
| 2.210                   | 2.210          | –             |
| 2.486                   | 2.486          | –             |
| 2.693                   | 2.693          | –             |
| 2.969                   | 2.969          | –             |
| 3.107                   | 3.107          | –             |
| 3.245                   | 3.245          | –             |
| 3.384                   | 3.384          | –             |
| 3.522                   | 3.522          | –             |
| 3.729                   | 3.729          | –             |
| 3.867                   | 3.867          | –             |
| 4.005                   | 4.005          | –             |

The interplay of the overlap part (blue) and the phase part (green) of the coherent term in the NEMol-ansatz is illustrated in FIG. S11 for two individual NEMol-grid points. Since we are forming the product of the overlap and the phase the overall coherent term (red) and thus the frequencies observed are higher than for the individual contributions. The oscillating electric field of the applied pulse and its Fourier transformed are shown in black.

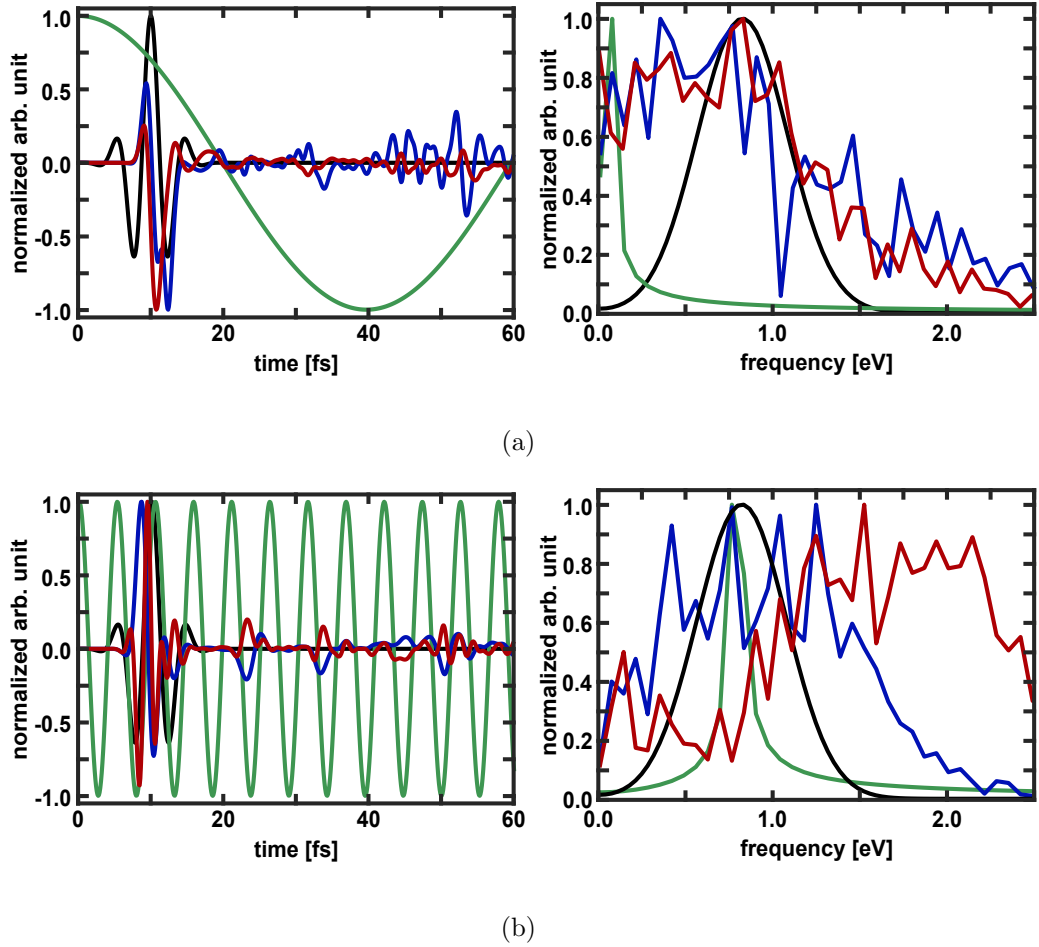

FIG. S11. Temporal evolution and Fourier transformation of Two-times the real-valued part of the overlap term (blue), the phase term (green) and the complete coherence term (red) for the (a) grid-window containing the CoIn and (b) a grid-window near the CoIn (one step to larger  $\alpha$  values). In the simulation the influence of a few-cycle IR laser pulse (black) is taken into account.

#### IV. INFLUENCE OF THE TDM ON THE WAVEFORM CONTROL

As shown in our previous work<sup>S22</sup> the interplay of the NAC's and the TDM along the direction of the motion of the wavepacket determines which CEP dependency is observed for the population. Therefor we want to examine the influence of the chosen transition dipole moment itself on the CEP-control schema regarding the population  $P_{D0}(t, \phi)$  and the asymmetry of the nuclei  $AN(t, \phi)$ . The temporal evolution of  $\Gamma(t)$  and the CEP dependent population  $P_{D0}(t, \phi)$  at 20 fs determined for the  $y$ -component, the  $z$ -component and the absolute value of the transition dipole moment are shown in FIG. S12.

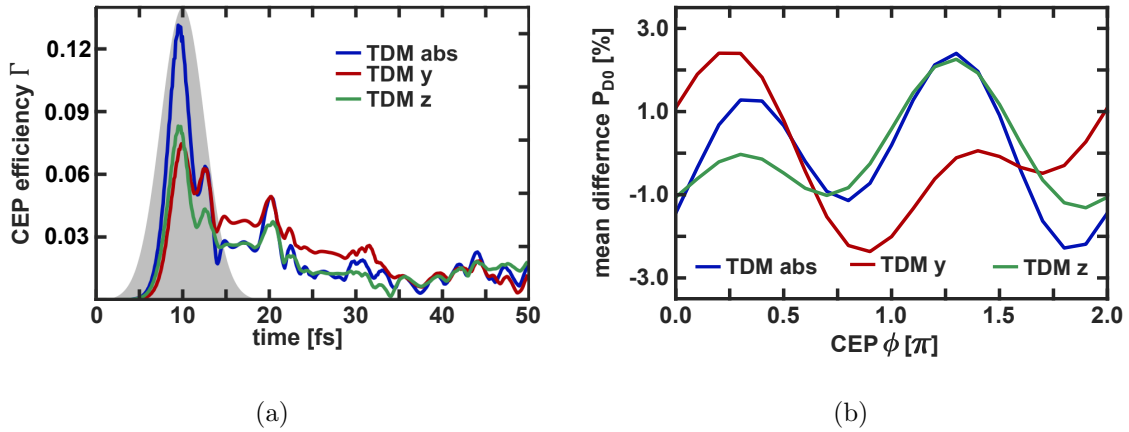

FIG. S12. (a) Temporal evolution of the CEP efficiency  $\Gamma(t)$  after  $t_0 = 10$  fs calculated with the absolute value, the  $y$ - and the  $z$ -component of the transition dipole moment. The envelope of the IR-pulse is indicated in grey. (b) Mean difference of the CEP-dependent populations  $P_{D0}(t, \phi)$  at 20 fs.

For all three types of the used transition dipole moment the general shape of  $\Gamma(t)$  is almost identical and only the magnitude is varying. During the pulse the absolute value of the TDM has the highest CEP efficiency. After the pulse  $\Gamma(t)$  obtained with the  $y$ -component is up to 35 fs the largest one and the CEP-efficiency obtained with the  $z$ -component is the smallest one both compared to the absolute value case. After 35 fs all three cases are nearly the same. In order to analyze the CEP-dependence of the population  $P_{D0}(t, \phi)$  (see FIG. 12(b)), its mean difference is recorded at 20 fs for all three types of transition dipole moment. Again the mean difference of the population is chosen for better visualization. The cases using the  $z$ -component (green) and the absolute value (blue) show a very similar CEP-dependence with a sinusoidal oscillation and a periodicity of approximately  $\pi$ . The population  $P_{D0}(t, \phi)$

calculated with the  $y$ -component (red) also shows a sinusoidal form but the periodicity tends more towards  $2\pi$ . This in indication, that an interference process participates in the overall process as expected. The maximal asymmetry of the nuclei  $AN_{max}(t)$  as function of time and the CEP-dependent asymmetry of the nuclei  $AN(t, \phi)$  at 30 fs are depicted in FIG. S13.

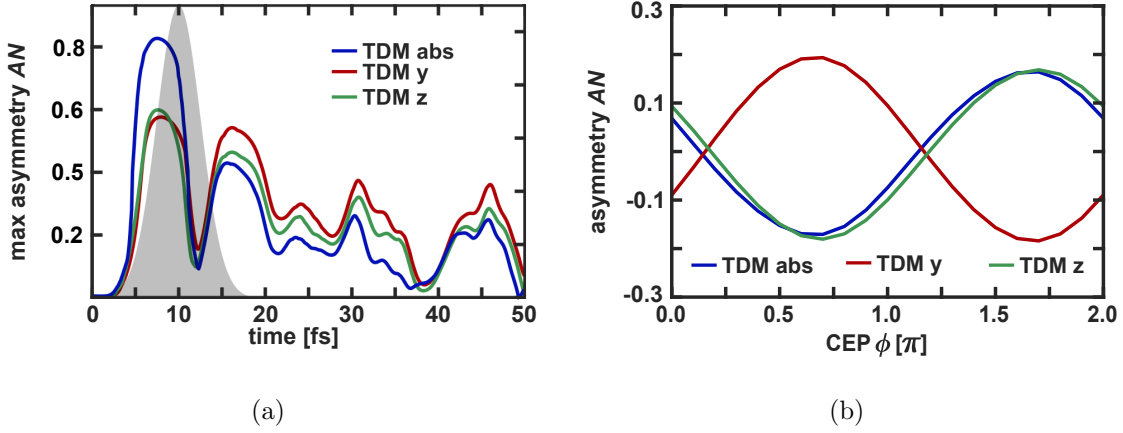

FIG. S13. (a) Temporal evolution of the maximal asymmetry of the nuclei  $AN_{max}(t)$  after  $t_0 = 10$  fs calculated with the absolute value, the  $y$ - and the  $z$ -component of the transition dipole moment. The envelope of the IR-pulse is indicated in grey. (b) The CEP-dependent asymmetry parameter  $AN(t, \phi)$  for 30 fs.

There is nearly no difference in the general shape of  $AN_{max}(t)$  regarding the used type of the transition dipole moment. Again the magnitude is the only difference. During the pulse  $AN_{max}(t)$  obtained with the absolute value (blue) is the largest. After the pulse the maximal asymmetry of the nuclei calculated with the  $y$ -component (red) is the largest one. The other two cases ( $z$ -component (green) absolute value (blue)) only differ in the time window from 20 fs to 35 fs. The mean difference of the CEP-dependent asymmetry parameter  $AN(t, \phi)$  is shown at 30 fs in FIG. 13(b). All three types of transition dipole moment show a sinusoidal oscillation with a periodicity of  $2\pi$ . For the case using the  $y$ -component (red) a phase shift of  $\pi$  with respect to the other two (blue and green) is observed.

## REFERENCES

- [S1]B. Podolsky, “Quantum-mechanically correct form of hamiltonian function for conservative systems,” *Physical Review* **32**, 812–816 (1928).
- [S2]E. B. Wilson, J. C. Decius, and P. C. Cross, *Molecular Vibrations: The Theory of Infrared and Raman Vibrational Spectra* (Dover Publ., 1980).
- [S3]L. Schaad and J. Hu, “The schrödinger equation in generalized coordinates,” *Journal of Molecular Structure: THEOCHEM* **185**, 203 – 215 (1989).
- [S4]S. Thallmair, M. K. Roos, and R. de Vivie-Riedle, “Design of specially adapted reactive coordinates to economically compute potential and kinetic energy operators including geometry relaxation,” *The Journal of Chemical Physics* **144**, 234104 (2016).
- [S5]D. R. Yarkony, “Diabolical conical intersections,” *Reviews of Modern Physics* **68**, 985–1013 (1996).
- [S6]M. Baer, “Introduction to the theory of electronic non-adiabatic coupling terms in molecular systems,” *Physics Reports* **358**, 75 – 142 (2002).
- [S7]A. Hofmann and R. de Vivie-Riedle, “Adiabatic approach for ultrafast quantum dynamics mediated by simultaneously active conical intersections,” *Chemical Physics Letters* **346**, 299 – 304 (2001).
- [S8]W. Domcke and G. Stock, *Advances in Chemical Physics* (John Wiley & Sons, Ltd, 2007) pp. 1–169.
- [S9]H. Tal-Ezer and R. Kosloff, “An accurate and efficient scheme for propagating the time dependent schrödinger equation,” *The Journal of Chemical Physics* **81**, 3967–3971 (1984).
- [S10]B. O. Roos, “The complete active space Self-Consistent field method and its applications in electronic structure calculations: Ab initio methods in quantum chemistry part 2,” in *Advances in Chemical Physics*, *Advances in Chemical Physics*, Vol. 41, edited by K. P. Lawley (John Wiley & Sons, Inc., Hoboken, NJ, USA, 1987) pp. 399–445.
- [S11]B. O. Roos, P. R. Taylor, and P. E. M. Sigbahn, “A complete active space SCF method (CASSCF) using a density matrix formulated super-CI approach,” *Chemical Physics*. **48**, 157–173 (1980).
- [S12]H.-J. Werner, P. J. Knowles, G. Knizia, F. R. Manby, M. Schütz, P. Celani, T. Korona, R. Lindh, A. Mitrushenkov, G. Rauhut, K. R. Shamasundar, T. B. Adler, R. D. Amos,

- A. Bernhardsson, A. Berning, D. L. Cooper, M. J. O. Deegan, A. J. Dobbyn, F. Eckert, E. Goll, C. Hampel, A. Hesselmann, G. Hetzer, T. Hrenar, G. Jansen, C. Köppl, Y. Liu, A. W. Lloyd, R. A. Mata, A. J. May, S. J. McNicholas, W. Meyer, M. E. Mura, A. Nicklass, D. P. O'Neill, P. Palmieri, D. Peng, K. Pflüger, R. Pitzer, M. Reiher, T. Shiozaki, H. Stoll, A. J. Stone, R. Tarroni, T. Thorsteinsson, and M. Wang, "MOLPRO, version 2012.1, a package of ab initio programs," (2012).
- [S13]H.-J. Werner, P. J. Knowles, G. Knizia, F. R. Manby, and M. Schütz, "Molpro: a general-purpose quantum chemistry program package: Molpro," *WIREs Computational Molecular Science* **2**, 242–253 (2012).
- [S14]R. Jost, J. Nygard, A. Pasinski, and A. Delon, "The photodissociation threshold of NO<sub>2</sub>: Precise determination of its energy and density of states," *The Journal of Chemical Physics* **105**, 1287–1290 (1996).
- [S15]W. C. Bowman and F. C. De Lucia, "The millimeter and submillimeter spectrum of NO<sub>2</sub>: A study of electronic effects in a nonsinglet light asymmetric rotor," *The Journal of Chemical Physics* **77**, 92–107 (1982).
- [S16]A. Delon, R. Jost, and M. Jacon, "Laser induced dispersed fluorescence spectroscopy of 107 vibronic levels of NO<sub>2</sub> ranging from 12000 to 17600 cm<sup>-1</sup>," *The Journal of Chemical Physics* **114**, 331–344 (2001).
- [S17]M. Richter, F. Bouakline, J. González-Vázquez, L. Martínez-Fernández, I. Corral, S. Patchkovskii, F. Morales, M. Ivanov, F. Martín, and O. Smirnova, "Sub-laser-cycle control of coupled electron–nuclear dynamics at a conical intersection," *New Journal of Physics* **17**, 113023 (2015).
- [S18]G. A. Worth and L. S. Cederbaum, "Beyond born-oppenheimer: Molecular dynamics through a conical intersection," *Annual Review of Physical Chemistry* **55**, 127–158 (2004), pMID: 15117250.
- [S19]H.-J. Werner and W. Meyer, "MCSCF study of the avoided curve crossing of the two lowest <sup>1</sup>Σ<sup>+</sup> states of LiF," *The Journal of Chemical Physics* **74**, 5802–5807 (1981).
- [S20]E. S. Kryachko and D. R. Yarkony, "Diabatic bases and molecular properties," *International Journal of Quantum Chemistry* **76**, 235–243 (2000).
- [S21]S. Thallmair, M. K. Roos, and R. de Vivie-Riedle, "Molecular features in complex environment: Cooperative team players during excited state bond cleavage," *Structural Dynamics* **3**, 043205 (2016).

[S22]F. Schüppel, T. Schnappinger, L. Bäuml, and R. de Vivie-Riedle, “Waveform control of molecular dynamics close to a conical intersection,” (2020), The Journal of Chemical Physics (accepted).
